# Supplementary material for: Post-quantum Zero Knowledge in Constant Rounds
Source: arXiv:1912.04769 source file (2020-04-20)
Supplement: Supplementary file 1 [file appendix.tex]

\section{Appendix}

\omri{Note: Refer to previous proofs, and explain that whenever we use the ZK property of the argument, we are going to: (1) assume towards contradiction that there's a distinguisher that distinguishes between simulated and real argument. (2) if there is such a distinguisher, it distinguishes with some non-negligible advantage $\epsilon$. (3) Now, consider the partially simulated distribution, the simulator halts after a number of steps that's proportional to $\epsilon$, note that its statistical distance from the fully simulated interaction is less then $\frac{\epsilon}{2}$. (4) Note that the distinguisher can distinguish between the partially simulated interaction and the real interaction with advantage at least $\frac{\epsilon}{2}$, and this time, both distributions can be generated in polynomial time.}

\begin{claim}[Coin-Flipping Simulator Runs in Expected Polynomial Time]\label{claim:cf_sim_time}
	There's a fixed polynomial $q(\cdot)$ such that for every polynomial-size quantum adversary $\cfmA = \{ \cfmA_\secp, \rho_\secp \}_{\secp \in \Nat}$ (and string $r\in \{ 0, 1 \}^k$), the expected running time of the simulation $\cfS(r, \cfmA_\secp, O_{\rho_\secp})$ is $q(|\cfmA_\secp|)$.
\end{claim}
